# Supplementary material for: 3D tracking of particles in a dusty plasma by laser sheet tomography
Source: arXiv:2302.12975 ancillary file (2023-06-04)
Supplement: Supplementary file 1 [file trackingdemo__1_.pdf]

# tracking\_demo

February 22, 2023

```
[1]: from __future__ import division, unicode_literals, print_function # for
      →compatibility with Python 2 and 3

import matplotlib as mpl
import matplotlib.pyplot as plt
import numpy as np
import pandas as pd
from pandas import DataFrame, Series # for convenience
import numpy as np
import numpy.fft as fft
import pims

import trackpy as tp
# change the following to %matplotlib notebook for interactive plotting
%matplotlib inline
import os
from PIL import Image
import time
```

```
[12]: pathr = r'D:\2022-10-3-nomag'
      filename = "0.1Pa0.6V250mV50HZ_1000"
      # specify your cine file's location here
      frames = (pims.open('{}/{}.cine'.format(pathr,filename)))
```

```
[69]: # define the class to handle 3d frame sequences. Input
      class CineToND(pims.FramesSequenceND):
          @property
          def pixel_type(self):
              return self.type
          def __init__(self, frames,fps,beginframe = None,numslides = None):
              """
              frames: pims.frame object, which you loaded your 2D frame
              fps: frames per bundle
              beginframe: the index of the beginning frame for each bundle.
              If none, will automatically infer by default
              numslides: how many slides to keep in each bundle.
```

*Discard the frames on the beginning and ending of each bundle,  
→symmetrically.*

```
'''
if numslides == None:
    numslides = fps
t_1 = 1
if beginframe == None:
    beginframe = np.argmax([frames[i].max() for i in range(20)])
    beginframe = (beginframe - numslides//2) % fps
elif beginframe == 0:
    t_1 = 0
try:
    self.type = frames.pixel_type
except:
    self.type = str(frames.dtype)
super().__init__() # properly initialize
self._init_axis('y', frames.shape[1])
self._init_axis('x', frames.shape[2])
self._init_axis('z', numslides)
self._init_axis('t', frames.shape[0]//fps-t_1)
self._register_get_frame(self.get_frame_2D, 'yx')
self.bundle_axes = 'zyx' # set default value
self.iter_axes = 't' # set default value
self.frames = frames
self.fps = fps
self.beginframe = beginframe
def get_frame_2D(self, **ind):
    t = ind['t']
    z = ind['z']

    return self.frames[t*self.fps + self.beginframe + z]
framesND = CineToND(frames,20,numslides = 8)
```

```
[19]: # Use trackpy to track particles
nparticles = 11
features = tp.batch(framesND, diameter=(3,3,3),separation=(2.5,2.5,2.5),
                    topn =nparticles,characterize = 0,engine='numba',
                    smoothing_size = 0,minmass = 99,preprocess = False)
```

```
[3]: '''
Use SPIFF to correct pixel-locking
'''
class IronTransform:
    def fit(self, data, weights = 'fuck'):
        if type(weights) == str:
            weights = np.ones(len(data))
            weights = weights / weights.sum()
```

```

    sorter = np.argsort(data)
    self.x = data[sorter]
    self.y = np.cumsum(weights[sorter])/2.
    return self

    def transform(self, data):
        return np.interp(data, self.x, self.y)

def fixsubpical(x):
    pixal = np.round(x)
    subpixal = x - pixal
    sign = np.sign(subpixal)
    np.abs(subpixal,out = subpixal)
    iron = IronTransform().fit(subpixal)
    fixedpixal = iron.transform(subpixal)
    return pixal + sign*fixedpixal

linked.loc[:, 'z'] = fixsubpical(linked.z.values)
linked.loc[:, 'x'] = fixsubpical(linked.x.values)
linked.loc[:, 'y'] = fixsubpical(linked.y.values)

'''linked.loc[linked.mass>150, 'x'] = fixsubpical(linked[linked.mass>150].x.
→values)
linked.loc[linked.mass>150, 'y'] = fixsubpical(linked[linked.mass>150].y.values)
linked.loc[linked.mass>150, 'z'] = fixsubpical(linked[linked.mass>150].z.values)
linked.loc[linked.mass<=150, 'x'] = fixsubpical(linked[linked.mass<=150].x.values)
linked.loc[linked.mass<=150, 'y'] = fixsubpical(linked[linked.mass<=150].y.values)
linked.loc[linked.mass<=150, 'z'] = fixsubpical(linked[linked.mass<=150].z.
→values)'''
#linked.to_csv('{} / {}.csv'.format(pathr, filename))

```

```

[907]: #link particles by predicting future positions parabolically
import trackpy as tp
from trackpy.predict import *

class _ParaPredict(NullPredict):
    def __init__(self, span=2):
        if span != 2:
            raise ValueError('Parabolic predictor, span must be 2!')
            """Use the 'span'+1 most recent frames to make a velocity field."""
            self.recent_frames = deque([], span + 1)

    def state(self):
        return list(self.recent_frames)

    def _compute_velocities(self, frame):
        """Compute velocity field based on a newly-tracked frame."""

```

```

pframe = frame.set_index('particle')
self.recent_frames.append(pframe)
#print(self.recent_frames)
dt = 1
    #dt = float(self.recent_frames[-1][self.t_column].values[0] -
    #          self.recent_frames[0][self.t_column].values[0])
if len(self.recent_frames) < 3:
    disps = self.recent_frames[-1][self.pos_columns].join(
        self.recent_frames[-1][self.pos_columns] -
        self.recent_frames[-1][self.pos_columns], rsuffix='_disp_').dropna()
    # Compute velocity field
else:
    disps = self.recent_frames[-1][self.pos_columns].join(
        1.8* self.recent_frames[-1][self.pos_columns] -
        2.6 *self.recent_frames[1][self.pos_columns] +
        0.8 *self.recent_frames[0][self.pos_columns], rsuffix='_disp_').
→dropna()
    positions = disps[self.pos_columns]
    vels = disps[[cn + '_disp_' for cn in self.pos_columns]] / dt
    # 'vels' will have same column names as 'positions'
    vels = vels.rename(columns=lambda n: n[:-6])
    #print(positions, vels)
    return dt, positions, vels
class ParabolicPredict(_ParaPredict):
    """Predict a particle's position based on the most recent nearby velocity.

    Parameters
    -----
    initial_guess_positions : Nxd array, optional
    initial_guess_vels : Nxd array, optional
        If specified, these initialize the velocity field with velocity
        samples at the given points.
    span : integer, default 1
        Compute velocity field from the most recent span+1 frames.
    """

    def __init__(self, initial_guess_positions=None,
                 initial_guess_vels=None, span=2):
        super().__init__(span=span)
        if initial_guess_positions is not None:
            self.use_initial_guess = True
            self.interpolator = NearestNDInterpolator(
                np.asarray(initial_guess_positions),
                np.asarray(initial_guess_vels))
        else:
            self.use_initial_guess = False

```

```

def observe(self, frame):
    dt, positions, vels = self._compute_velocities(frame)
    #damn.append(positions)
    #vellist.append(vels)
    if self.use_initial_guess:
        self.use_initial_guess = False
    else:
        if positions.values.shape[0] > 0:
            self.interpolator = NearestNDInterpolator(positions.values[:,::-1],
→-1],
                                                    vels.values[:,::-1])

        else:
            # Sadly, the 2 most recent frames had no points in common.
            warn('Could not generate velocity field for prediction: no_
→tracks')

            def null_interpolator(*x):
                return np.zeros((len(x),))

            self.interpolator = null_interpolator

def state(self):
    return {'recent_frames': list(self.recent_frames),
            'interpolator': self.interpolator,
            'using_initial_guess': self.use_initial_guess,
            }

def predict(self, t1, particles):
    poslist, tlist = zip(*[(p.pos, p.t) for p in particles])
    positions = np.array(poslist)
    times = np.array(tlist)
    result = (positions + self.interpolator(positions) *
              np.tile(.62*(t1 - times), (positions.shape[1], 1)).T)
    return result

pred = ParabolicPredict()
#pred = NearestVelocityPredict()
#features = data2[(data2.frame > -3000) & (data2.frame < 100000)]
linked = pd.concat(pred.link_df_iter((frame for fnum, frame in features.
→groupby('frame')),
                                14,memory=3, pos_columns=['x', 'y', 'z'],a
                                daptive_step = 0.8, adaptive_stop = 3))

```

Frame 12971: 11 trajectories present.

```

[22]: def microprocess_xyz(df, z0 = 520, y0 = 500, xperpixal = 0.149, zperpixal = 0.
→32):
    '''

```

```

df: your linked dataframe
z0, y0: see text
xperpical: the scale in mm per pixel in xy plane at the center
zperpical: the scale in mm per slide in z at the center
'''

df.x -= df.x.mean()
df.y -= df.y.mean()
df.z -= df.z.mean()
df['xmm'] = (df.x) * xperpical
df['ymm'] = (df.y) * xperpical
df['zmm'] = (df.z) * zperpical * (y0 + df.ymm) / y0
df.xmm = df.xmm * (z0 - df.zmm) / z0
df.ymm = df.ymm * (z0 - df.zmm) / z0
def microprocess_t(df,dz = 6.4):
    '''
    dz: the slope of the laser height z per cycle.
    '''

    ex = 20
    #tish = df.stack().reset_index()
    tish = df.copy()
    tish.frame = tish.frame*ex + round(tish.z/dz*ex).astype(int)
    frame = tish.frame
    new_data = tish.set_index(['frame', 'particle']).unstack()
    new_data = new_data.reindex(range(frame.min(),frame.max()+1)).
→interpolate('akima')
    tish = new_data.loc[list(range(ex//2,frame.max()-ex,ex))].stack().
→reset_index()
    tish.frame = tish.frame // (ex)
    #####
    return tish.set_index(['frame', 'particle']).unstack()

```
